# Supplementary material for: Frequency-Aware Reconstruction of Fluid Simulations with Generative Networks
Source: arXiv:1912.08776 source file (2019-12-18)
Supplement: Supplementary file 1 [file appendix.tex]

\section{Appendix}
\label{sec:appendix}

\section{Properties of Fourier Loss}
Let $\vec{x}, \vec{y}$ be arbitrary tensors of arbitrary, but equal dimensions. For 
$$d(\vec{x}, \vec{y}) = L_{fol}(\vec{x}, \vec{y}) = \sum_b w_b \cdot L_{norm}(b) = \sum_b w_b \cdot \left \lVert |FT(\vec{x})_b - FT(\vec{y})_b| \right \rVert_1, w_b \in \mathbb{R}^+$$
to be a proper metric (distance) it has to fulfill:
\begin{enumerate}
	\item $d(\vec{x},\vec{y}) \geq 0$ (non-negativity)
	\item $d(\vec{x},\vec{y}) = 0 \Leftrightarrow \vec{x} = \vec{y}$ (identity of indiscernibles)
	\item $d(\vec{x},\vec{y}) = d(\vec{y},\vec{x})$ (symmetry)
	\item $d(\vec{x},\vec{z}) \leq d(\vec{x},\vec{y}) + d(\vec{y},\vec{z})$ (triangle inequality)
\end{enumerate}

Most properties follow from the fact that we use a weighted sum of $\ell_1$-norms. A full list of proofs is given for completeness in the following subsections.

\subsection{Non-Negativity}
We have $w_b > 0$ by definition and the $\ell_1$-norm is non-negative because it is a proper norm. The fact that a sum of non-negative values is always non-negative concludes the proof.
\begin{align}
d(\vec{x}, \vec{y}) &= \sum_b \underbrace{w_b}_{> 0} \cdot \underbrace{\left \lVert |FT(\vec{x})_b - FT(\vec{y})_b| \right \rVert_1}_{\geq 0} \geq 0
\end{align}

\subsection{Identity of Indiscernibles}
We show the two implications separately:
\begin{itemize}
	\item $\vec{x} = \vec{y} \Rightarrow d(\vec{x},\vec{y}) = 0$:
		
		We have $FT(\vec{x})_b = FT(\vec{y})_b$ since $\vec{x} = \vec{y}$ and therefore $\left \lVert |FT(\vec{x})_b - FT(\vec{y})_b| \right \rVert_1 = 0$.
		\begin{align}
			d(\vec{x}, \vec{y}) &= \sum_b w_b \cdot \underbrace{\left \lVert |FT(\vec{x})_b - FT(\vec{y})_b| \right \rVert_1}_{= 0} = 0
		\end{align}
		
	\item $d(\vec{x},\vec{y}) = 0 \Rightarrow \vec{x} = \vec{y}$:
	
		Since all $w_b>0$ and all summands are positive, we know that all summands have to equal 0. This means that $FT(\vec{x})_b = FT(\vec{y})_b$, for all $b$. Since the Fourier transform is invertible this implies $\vec{x} = \vec{y}$.
	\end{itemize}

\subsection{Symmetry}
We can use the fact that the complex norm is a norm to get 

\begin{align}
\left \lVert |FT(\vec{x})_b - FT(\vec{y})_b| \right \rVert_1 
&= \left \lVert |-1| \cdot |FT(\vec{x})_b - FT(\vec{y})_b| \right \rVert_1 \\
&= \left \lVert |(-1) \cdot (FT(\vec{x})_b - FT(\vec{y})_b)| \right \rVert_1 \\
&= \left \lVert |FT(\vec{y})_b - FT(\vec{x})_b)| \right \rVert_1
\end{align}

which shows the symmetry:
\begin{align}
			d(\vec{x}, \vec{y}) &= \sum_b w_b \cdot \left \lVert |FT(\vec{x})_b - FT(\vec{y})_b| \right \rVert_1 = \sum_b w_b \cdot \left \lVert |FT(\vec{y})_b - FT(\vec{x})_b| \right \rVert_1 = d(\vec{x}, \vec{y}).
\end{align}

\subsection{Triangle Inequality}

\begin{align}
	d(\vec{x}, \vec{y}) + d(\vec{y}, \vec{z}) &= \sum_b w_b \cdot \left \lVert |FT(\vec{x})_b - FT(\vec{y})_b| \right \rVert_1 + \sum_b w_b \cdot \left \lVert |FT(\vec{y})_b - FT(\vec{z})_b| \right \rVert_1 \\
	&= \sum_b w_b \cdot \left( \lVert |FT(\vec{x})_b - FT(\vec{y})_b|  \rVert_1 + \lVert |FT(\vec{y})_b - FT(\vec{z})_b|  \rVert_1 \right) \\
	&\geq \sum_b w_b \cdot \lVert |FT(\vec{x})_b - FT(\vec{z})_b| \rVert_1 \\
	&=	d(\vec{x}, \vec{z})
\end{align}

In the inequality we used the triangle inequality for the complex norm and the definition of the $\ell_1$ norm.
